# Supplementary material for: Training Over a Distribution of Hyperparameters for Enhanced Performance and Adaptability on Imbalanced Classification
Source: arXiv:2410.03588 source file (2024-10-04)
Supplement: Supplementary file 1 [file sec_appendix_margins.tex]

% In addition to AUROC and accuracy, another important aspect of a model's performance is the distance of the sample to the decision boundary, or the margins of the samples. In this document, we compare the margins of our Baseline and LCT model.

\section{Analysis of VS loss hyperparameters}
In this section, we examine how the hyperparameters of the VS loss and the imbalance ratio $\beta$ affect the decision boundaries and loss landscape of a binary classifier.

\subsection{Decision Boundary}
\label{sec:zdecision_boundary}
We first observe that the hyperparameters of VS loss do not affect the decision boundary. The decision boundary is the hyperplane $g(\mathbf{z})=\mathbf{\mathbf{w}\cdot\mathbf{z}} + w_0=0$ such that $\hat{y}=+$ if $g(\mathbf{z})>0$ and $\hat{y}=-$ if $g(\mathbf{z})\leq0$. The decision boundary is solely determined by the user via the threshold $t$ and the hyperparameters of the loss function have no direct effect on this. 

\subsection{Break-even points}
T hyperparameter values do, however, affect the loss landscape. To study this, we consider the break-even points, or the points on the $(z_-, z_+)$ plane such that 

\begin{align}
\ell(-, \bz) = \ell(+, \bz).
\end{align}

From \cref{eq:vs0,eq:vs1}, we see this happens when

\begin{align}
    z_+/\beta^\gamma - (z_- + \tau \log\beta) &= (z_- + \tau \log\beta) - z_+/\beta^\gamma
\end{align}

which simplifies to 

\begin{align}
    z_+ &= \beta^\gamma z_- + \beta^\gamma(\tau \log\beta)
\end{align}

In ~\cref{fig:break_even}, we plot the difference $\ell(+,\mathbf{z}) - \ell(-,\mathbf{z})$ over the plane $\mathbf{z}$. The break-even points, or the points of $\mathbf{z}$ where $\ell(1,\mathbf{z}) = \ell(0,\mathbf{z})$, are shown in white. From the top row, we see that when $\gamma=0$ (that is, when the logits are scaled equally in the loss function), increasing $\tau$ is equivalent to shifting the line of break-even points, since $\tau$ controls bias on the logits. From the left column, we see that when $\tau=0$ (no bias on the logits), increasing $\gamma$ equates to rotating the line of break-even points, since different values of $\gamma$ scale the logits differently.

\begin{figure}[h]
    \centering
    \includegraphics[width=0.8\linewidth]{results_07_02/break_even_sns.png}
    \caption{Effect of hyperparameter values on $\ell(+,\mathbf{z})- \ell(-,\mathbf{z})$ over $z_-, z_+ \in [-5, 5]$ for $\beta=10$. Rows and columns show different values for $\gamma$ and $\tau$ respectively. White lines represent break-even points.}
    \label{fig:break_even}
\end{figure}

\subsection{Simplifying logits for VS loss models}
In this section, we explore whether the 2D logits $\mathbf{z}$ from binary models trained with VS loss can be expressed in one dimension, $\theta$. To do this, we observe that models trained with VS loss will only produce logits that fall along the line through the origin and in the direction of the vector $\bn = (-1, \beta^{-\gamma})$. To understand this, first observe that ~\cref{eq:vs0,eq:vs1} show that the loss does not depend on the component perpendicular to this line. Then the logits start close to zero during training (because the weights are initialized to small random values) and the gradient will only move them along this line since the gradient of the loss in the direction orthogonal to it is zero. Thus, we only need to study the component of $\bz$ in the direction of $\bn$. This is defined as follows,
\begin{align}
\theta = \bu \cdot \bz \spacetext{, where} \bu = \bn / \|\bn\| \label{eq:theta_calc}
\end{align}
is the unit-norm version of $\bn$. 

In~\cref{fig:z_and_theta_cifar,fig:z_and_theta_melanoma} we find that this assumption holds for both Baseline and LCT models on binary subsets of CIFAR10 and Baseline models on the Melanoma dataset; however, this does not hold for LCT models on the Melanoma dataset. Notice how the clouds of logits fall along the blue line for all the models in~\cref{fig:z_and_theta_cifar} and all the Baseline models in~\cref{fig:z_and_theta_melanoma}; however, the point clouds for the LCT models on the Melanoma dataset do not follow the line of the logits and are much more spread out.

We hypothesize that this might be because the models trained on the Melanoma dataset have not been trained as long as the models trained on the CIFAR datasets. To test this hypothesis, we analyze point clouds for the CIFAR dataset from earlier epochs in ~\cref{fig:zs_during_training}. We find that early in training the outputs don't fall along the logit line (see left column of~\cref{fig:zs_during_training}); however, as training continues, the logits align better with the line.  

Although these findings indicate that the $\theta$ assumption may hold for a later epoch on the Melanoma models, we know that the gap between Baseline and LCT is largest for the Melanoma dataset. Thus, we propose continuing to study the models trained to this point, but do not use $\theta$ since this is an invalid assumption in this case.

\begin{figure}
    \centering
    \includegraphics[width=0.9\linewidth]{results_07_02/z_plot_cifar_baseline_100.png}
    \includegraphics[width=0.9\linewidth]{results_07_02/z_plot_cifar_lct_100.png}
    \caption{Plots of $\mathbf{z}$ outputs for 12 Baseline and 12 LCT models trained on the Automobile/bird subset of CIFAR10 with $\beta=100$. Blue dots and orange dots represent $\mathbf{z}$ outputs for $-$ and $+$ samples respectively. Blue line is the line that we would expect the logits to fall on (line through the origin in the direction of $\bn = (-1, \beta^{-\gamma})$). Green and red lines are decision boundaries for $t=0.5$ and $t=0.95$ respectively. Orange line is the break-even line in the loss landscape. \textbf{All models trained on CIFAR subsets give $\mathbf{z}$ outputs that fall along the logit line.}}
    \label{fig:z_and_theta_cifar}
\end{figure}

\begin{figure}
    \centering
    \includegraphics[width=0.9\linewidth]{results_07_02/z_plot_baseline_200.png}
    \includegraphics[width=0.9\linewidth]{results_07_02/z_plot_lct_200.png}
    \caption{Plots of $\mathbf{z}$ outputs for 12 Baseline and 12 LCT models trained on the Melanoma dataset with $\beta=200$. Blue dots and orange dots represent $\mathbf{z}$ outputs for $-$ and $+$ samples respectively. Blue line is the line that we would expect the logits to fall on (line through the origin in the direction of $\bn = (-1, \beta^{-\gamma})$). Green and red lines are decision boundaries for $t=0.5$ and $t=0.95$ respectively. Orange line is the break-even line in the loss landscape. \textbf{Baseline models trained on the Melanoma subsets give $\mathbf{z}$ outputs that fall along the logit line, but LCT models do not.}}
    \label{fig:z_and_theta_melanoma}
\end{figure}

\begin{figure}
    \centering
    \includegraphics[width=0.9\linewidth]{results_07_02/z_plot_cifar_lct_100_epochs.png}
    \caption{Plots of $\mathbf{z}$ outputs for 3 LCT models evaluated at 4 different epochs. Models were trained on CIFAR10 automobile/bird with $\beta=100$. Blue dots and orange dots represent $\mathbf{z}$ outputs for $-$ and $+$ samples respectively. Blue line is the line that we would expect the logits to fall on (line through the origin in the direction of $\bn = (-1, \beta^{-\gamma})$). Green and red lines are decision boundaries for $t=0.5$ and $t=0.95$ respectively. Orange line is the break-even line in the loss landscape. \textbf{As models are trained longer, the $\mathbf{z}$ outputs align with the logit line better.} }
    \label{fig:zs_during_training}
\end{figure}

% Recall that in \cref{sec:decision_boundary} we found an equation that takes a softmax thershold $t$ and gives the hyperplane of the decision boundary in $\mathbf{z}$. We can extend this to find the threshold in $\theta_t$. To do this, find the point where the decision boundary intersects the line that the logits fall on. In other words, find the point where the following two lines intersect.

% \begin{align}
%     z_+ - z_- - \ln(\frac{t}{1-t}) = 0 \\
%     z_+ + \beta^{-\gamma}z_- = 0
% \end{align}

% This is 
% \begin{align}
%     \mathbf{z_t} &= \left(-\frac{\ln(\frac{t}{1-t})}{1+\beta^{-\gamma}}, \beta^\gamma \frac{\ln(\frac{t}{1-t})}{1+\beta^{-\gamma}}  \right).
% \end{align}

% Then use~\cref{eq:theta_calc} to compute the $\theta$ value of this point as
% \begin{align}
%     \theta_t &= \frac{2\ln(\frac{t}{1-t})}{(1+\beta^{-\gamma})\sqrt{1+\beta^{-2\gamma}}}
% \end{align}

% If $t=0.5$, the decision boundary on $\theta$ is $\theta_0=0$. 

\section{Results of Baseline and LCT}
In this paper we compare the best Baseline model and the best LCT model that were trained on the Melanoma dataset with $\beta=200$. We summarize the performance of both of these models in~\cref{tab:overall_results} in terms of AUROC and Balanced accuracy.

%We plot the histogram of $\theta$s for the test set for each of these models in ~\cref{fig:theta_dist}. Additionally, we find the threshold of $\theta$ that optimizes the balanced accuracy and plot this threshold (see ~\cref{sec:balanced_vs_overall} for more details about Balanced accuracy).

% \begin{figure}
%     \centering
%     \includegraphics[width=\linewidth]{results_07_02/best_thetas.png}
%     \caption{Distribution of $\theta$s for the best Baseline and best LCT model. For each model, we give the AUROC and the best balanced accuracy of the model.}
%     \label{fig:theta_dist}
% \end{figure}

\subsection{Balanced accuracy}

\begin{table}[]
    \centering
    \begin{tabular}{c|c|c|c}
        Model name & AUROC & Best $t$ & Balanced acc. at best $t$ \\
        \hline
        Baseline & 0.881 & 0.95 & 78.9 \\
        LCT & 0.906 & 0.98 & 82.3
    \end{tabular}
    \caption{Results for best Baseline and best LCT model. }
    \label{tab:overall_results}
\end{table}

\subsection{Margins}
In addition to AUROC and Balanced accuracy, we consider the distance of the points to the decision boundary or the margins. To do this, we choose the decision boundary to be the boundary that corresponds to the softmax threshold $t$ that gives the best balanced accuracy.

We first consider the margins in the model's output (logit) space. This is the signed distance between the model's outputs $\mathbf{z}$ and the decision boundary where the distance is positive if the sample is correctly classified and negative otherwise. Using the equation for a decision boundary (~\cref{eq:decision_boundary}) and the equation for the distance of a point from a line, we calculate the margin of a point $\mathbf{z}$ from a decision boundary with softmax threshold $t$ as follows.

\begin{align}
    m_z = \frac{y \left(-z_- + z_+ - \ln\left(\frac{t}{1-t}\right) \right)}{\sqrt{2}}
\end{align}

We show results of $m_z$ for both models in the top row of ~\cref{fig:margins_tp}. 

However, the margin in logit space is not particularly informative since the scale of the logits may differ from one model to another. For example, let $x$ be an input image and $x'$ be another slightly different input image. Suppose we feed both $x$ and $x'$ to a model A to get output $z_A$ and $z_A'$. The distance $||z_A - z_A'||$ depends on how sensitive model $A$'s outputs are to differences in the input $||x-x'||$. In particular, model A may have larger margins, but it could also be the case that $||z_A - z_A'|| >> ||z_B - z_B'||$, implying that model A is more sensitive to $||x-x'||$ than model B and the larger margins in $\mathbf{z}$ are not meaningful. Thus, we also estimate the distance to the decision boundary (\ie the margins) in data (input) space. To do this, we estimate the sensitivity of each sample's margin $m_z$ with respect to its inputs using a linear approximation of the network. Thus, we estimate the margin in $x$ space as follows.

\begin{align}
    m_x &\approx \frac{m_z}{\left|\left| \nabla_{x} m_z \right| \right|} \label{eq:approx_margin}
\end{align} 

\paragraph{Proof of Inequality}
In this paragraph we prove why \cref{eq:approx_margin} is only an approximate bound and not an inequality.

Let \bx\ be a data sample and let $m = \phi(\bx)$ be its margin. Let $\bx'$ be a perturbation of \bx\ and $m' = \phi(\bx')$.
Then, truncating the Taylor series of $\phi$ around \bx\ to the linear term yields
\[
m' - m \approx \nabla\phi(\bx) \cdot (\bx' - \bx)
\]
and therefore
\[
|m' - m| \approx |\nabla\phi(\bx) \cdot (\bx' - \bx)| \leq \|\nabla\phi(\bx)\|\ \|\bx' - \bx\|
\]
from the Cauchy-Schwarz inequality. Therefore, if $\|\nabla\phi(\bx)\| > 0$,
\[
\|\bx' - \bx\| \geq \frac{|m' - m|}{\|\nabla\phi(\bx)\|}
\]
approximately (\textbf{end of proof})

~\cref{fig:margins_tp} shows that the LCT model has larger margins $m_x$ on average than the Baseline model for both true positive and true negative samples. This suggests that LCT is more robust to perturbations in the data than Baseline models. This also implies that LCT's superior AUROC and Balanced accuracy performance is not a result of overfitting to the test set. However, LCT also has larger negative margins for the false positive and false negative samples. This implies that when LCT makes a wrong prediction, it is more confident in the prediction than Baseline, which is an undesirable property.

\begin{figure}
    \centering
    \includegraphics[width=\linewidth]{results_07_02/margins.png}
    \caption{Margins of baseline and LCT models. Top row is margins in logit space $m_z$. Bottom row is margins in data space $m_x$. $m_x$ is found by dividing $m_z$ by the norm of the gradient of $m_z$ with respect to the inputs. From left to right, columns show results for true positive, true negative, false positive, and false negative samples. Legend includes the mean of $m_z$, $\mu$. \textbf{LCT models have higher (better) margins for correct predictions and slightly lower (worse) margins for the incorrect predictions.}}
    \label{fig:margins_tp}
\end{figure}
